# Supplementary material for: A PMP-inspired Evaluation Framework for Assessing Deep-Learning Earth System Models
Source: arXiv:2604.06567 source file (2026-06-23)
Supplement: Supplementary file 1 [file 1_Supplementary_material.tex]

% \section{Supplementary Figures}

%%%%%%%%%%%%%%%%%%%%%%%% SI FIGURES  %%%%%%%%%%%%%%%%%%%%%%%%
\clearpage
\newpage
\setcounter{figure}{0}
\clearpage
% \appendix
\section{Supplementary Figures}
\setcounter{figure}{0}

% \subsection{Stability}
% %---------------------- FIGURE S1 --------------------------
% \clearpage
% \newpage
% \begin{figure}[h]
% %\captionsetup{textfont=largefont}
% \centering
% % TRIM = left, bottom, right, top
% % \renewcommand{\figurename}{Fig. S}
%     \centering
%     \includegraphics[width=0.7\textwidth]{Paper_figures/Stability.jpg}
% %     \includegraphics[width=0.8\linewidth,trim={0cm -0.5cm 0cm 0cm},clip]{ED_Fig_1_average.pdf}
% % \vspace*{0.0cm}
%     \caption{Comparing stable runs in NeuralGCM-precip (left) versus NeuralGCM-evap (right) for the period XX-XX-XX.}
%     \label{SIfig:stab}
% \end{figure}

\subsection{Climatology}
\label{SI:clim}
Metrics include mean climate for precipitation (pr), sea level pressure (psl), temperature (ta), and zonal (ua) and meridional winds (va).
    % \item For AI-based models, there are two versions: one for 1980–2005 and another for 1980–2014.
%---------------------- FIGURE S2 --------------------------
\begin{figure}[h]
    \centering
    \includegraphics[width=0.5\textwidth]{Paper_figures/clim_ACE_pr.jpg}
    \caption{Mean precipitation as simulated by ACE2 for the period 1981-2013. (a) Annual; Seasonal averages: (b) Winter, (c) Spring, (b) Summer, (b) Fall. }
    \label{SIfig:clim_ACE_pr}
\end{figure}

%---------------------- FIGURE S3 --------------------------
\begin{figure}[h]
    \centering
    \includegraphics[width=0.5\textwidth]{NERSC_figures/climatology/ACE2/psl_mon_ACE2-ERA5_amip_r1.198101-201312.AC.v20251103.png}
    \caption{Example of Mean psl - ACE 1981-2013.}
    \label{SIfig:clim_ACE_psl}
\end{figure}

% %---------------------- FIGURE S4 --------------------------
% \begin{figure}[h]
% % \renewcommand{\figurename}{Fig. S}
%     \centering
%     \includegraphics[width=1\textwidth]{NERSC_figures/potrait_mean_climate_global_mae.png}
%     \caption{Portrait plot for spatial Mean Absolute Error across different seasons. Negative normalized error indicates performance better than the multi-model median (like in \citep{Ullrich2025}.}
%     \label{SIfig:portrait_MAE}
% \end{figure}

%---------------------- FIGURE S4 --------------------------
\begin{figure}[h]
    \centering
    \includegraphics[width=0.4\textwidth]{Paper_figures/SI_ACE2_Ta_850_bias.jpg}
    \caption{ACE2 simulation of global annual mean for air temperature at 850 hPa compared to ERA5.}
    \label{SIfig:ACEbias_ta850}
\end{figure}

%---------------------- FIGURE S6 --------------------------
\begin{figure}[h]
    \centering
    \includegraphics[width=0.5\textwidth]{NERSC_figures/climatology/ACE2/pr_mon_ACE2-ERA5_amip_r1.198101-201312.AC.v20251103.png}
    \caption{Example of Mean precipitation  - ACE 1981-2013.}
    \label{SIfig:clim_ACE_pr}
\end{figure}

%---------------------- FIGURE S7 --------------------------

\begin{figure}[h]
    \centering
    \includegraphics[width=0.5\textwidth]{NERSC_figures/climatology/ACE2/psl_mon_ACE2-ERA5_amip_r1.198101-201312.AC.v20251103.png}
    \caption{Example of Mean psl - ACE 1981-2013.}
    \label{SIfig:clim_ACE_psl}
\end{figure}

\begin{figure}[h]
    \centering
    \includegraphics[width=0.5\textwidth]{NERSC_figures/climatology/ACE2/ta-200_mon_ACE2-ERA5_amip_r1.198101-201312.AC.v20251103.png}
    \caption{Example of Mean ta-200 - ACE 1981-2013.}
    \label{SIfig:clim_ACE_ta200}
\end{figure}

\begin{figure}[h]
    \centering
    \includegraphics[width=0.5\textwidth]{NERSC_figures/climatology/ACE2/ta-850_mon_ACE2-ERA5_amip_r1.198101-201312.AC.v20251103.png}
    \caption{Example of Mean ta-850 - ACE 1981-2013.}
    \label{SIfig:clim_ACE_ta850}
\end{figure}

\begin{figure}[h]
    \centering
    \includegraphics[width=0.5\textwidth]{NERSC_figures/climatology/ACE2/ua-200_mon_ACE2-ERA5_amip_r1.198101-201312.AC.v20251103.png}
    \caption{Example of Mean ua-200 - ACE 1981-2013.}
    \label{SIfig:clim_ACE_ua200}
\end{figure}

\begin{figure}[h]
    \centering
    \includegraphics[width=0.5\textwidth]{NERSC_figures/climatology/ACE2/ua-850_mon_ACE2-ERA5_amip_r1.198101-201312.AC.v20251103.png}
    \caption{Example of Mean ua-850 - ACE 1981-2013.}
    \label{SIfig:clim_ACE_ua850}
\end{figure}

\begin{figure}[h]
    \centering
    \includegraphics[width=0.5\textwidth]{NERSC_figures/climatology/ACE2/va-200_mon_ACE2-ERA5_amip_r1.198101-201312.AC.v20251103.png}
    \caption{Example of Mean va-200 - ACE 1981-2013.}
    \label{SIfig:clim_ACE_va200}
\end{figure}

\begin{figure}[h]
    \centering
    \includegraphics[width=0.5\textwidth]{NERSC_figures/climatology/ACE2/va-850_mon_ACE2-ERA5_amip_r1.198101-201312.AC.v20251103.png}
    \caption{Example of Mean va-850 - ACE 1981-2013.}
    \label{SIfig:clim_ACE_va850}
\end{figure}

\begin{figure}[h]
    \centering
    \includegraphics[width=0.5\textwidth]{NERSC_figures/climatology/NeuralGCM/ta-200_mon_NeuralGCM_amip_r1.198101-201312.AC.v20251027.png}
    \caption{Example of Mean ta-200 - NeuralGCM 1981-2013.}
    \label{SIfig:clim_NeuralGCM_ta200}
\end{figure}

\begin{figure}[h]
    \centering
    \includegraphics[width=0.5\textwidth]{NERSC_figures/climatology/NeuralGCM/ta-850_mon_NeuralGCM_amip_r1.198101-201312.AC.v20251027.png}
    \caption{Example of Mean ta-850 - NeuralGCM 1981-2013.}
    \label{SIfig:clim_NeuralGCM_ta850}
\end{figure}

\begin{figure}[h]
    \centering
    \includegraphics[width=0.5\textwidth]{NERSC_figures/climatology/NeuralGCM/ua-200_mon_NeuralGCM_amip_r1.198101-201312.AC.v20251027.png}
    \caption{Example of Mean ua-200 - NeuralGCM 1981-2013.}
    \label{SIfig:clim_NeuralGCM_ua200}
\end{figure}

\begin{figure}[h]
    \centering
    \includegraphics[width=0.5\textwidth]{NERSC_figures/climatology/NeuralGCM/ua-850_mon_NeuralGCM_amip_r1.198101-201312.AC.v20251027.png}
    \caption{Example of Mean ua-850 - NeuralGCM 1981-2013.}
    \label{SIfig:clim_NeuralGCM_ua850}
\end{figure}

\begin{figure}[h]
    \centering
    \includegraphics[width=0.5\textwidth]{NERSC_figures/climatology/NeuralGCM/va-200_mon_NeuralGCM_amip_r1.198101-201312.AC.v20251027.png}
    \caption{Example of Mean va-200 - NeuralGCM 1981-2013.}
    \label{SIfig:clim_NeuralGCM_va200}
\end{figure}

\begin{figure}[h]
    \centering
    \includegraphics[width=0.5\textwidth]{NERSC_figures/climatology/NeuralGCM/va-850_mon_NeuralGCM_amip_r1.198101-201312.AC.v20251027.png}
    \caption{Example of Mean va-850 - NeuralGCM 1981-2013.}
    \label{SIfig:clim_NeuralGCM_va850}
\end{figure}

\begin{figure}[h]
    \centering
    \includegraphics[width=0.5\textwidth]{NERSC_figures/climatology/NeuralGCM/zg-500_mon_NeuralGCM_amip_r1.198101-201312.AC.v20251027.png}
    \caption{Example of Mean zg-500 - NeuralGCM 1981-2013.}
    \label{SIfig:clim_NeuralGCM_zg500}
\end{figure}

\begin{figure}[h]
    \centering
    \includegraphics[width=0.5\textwidth]{NERSC_figures/climatology/NeuralGCM/psl_mon_NeuralGCM_amip_r1.198101-201312.AC.v20251027.png}
    \caption{Example of Mean precipitation  - NeuralGCM-precip.}
    \label{SIfig:clim_NeuralGCM_psl}
\end{figure}

%---------------------- FIGURE S5 --------------------------
\begin{figure}[h]
    \centering
    \includegraphics[width=1\textwidth]{Paper_figures/Portrait_MAE.png}
    \caption{Portrait plot for spatial Mean Absolute Error across different seasons. Negative normalized error indicates performance better than the multi-model median (like in \citep{Ullrich2025} and \citep{lee2024PMP}. The climatology metric is computed with respect to the observed climatological fields provided by the reference dataset product corresponding to each examined variable as reported in Table \ref{tab:models}. Grey cells correspond to not available variable output due to the specific model design.}
    \label{SIfig:portrait_MAE}
\end{figure}

\begin{figure}[h]
    \centering
    \includegraphics[width=1\textwidth]{Paper_figures/MJO_spectra_summer.jpg}
    \caption{MJO propagation metrics – wavenumber–frequency power spectra – from (a) obervations as from GPCP v1.3 (Huffman et al., 2001) and (b) ACE2, (c) NeuralGCM-evap and (d) NeuralGCM-precip. The EWR is defined as the ratio of eastward power (as the average power in the dashed box on the right) to westward power (as the average power in the dashed box on the left) from the 2-dimensional wavenumber–frequency power spectra of daily 10°N-–10°S averaged precipitation in May to October (shaded; mm$^2$d$^{−2}$). The average power spectrum over the period is computed as the average of the all the power spectra calculated for each year. The units of power spectra for the precipitation is mm$^2$d$^{−2}$) per frequency interval per wavenumber.}
    \label{SIfig:MJOprop_summer}
\end{figure}

\begin{figure}[h]
    \centering
    \includegraphics[width=1\textwidth]{Paper_figures/MJO_NDJFMA.png}
    \caption{MJO east–west power ratio (EWR; unitless) from CMIP6 models ( orange) compared to the Dl-ESMs (red) for boreal summer. The EWR corresponding to the observational dataset is shown in gray (GPCP v1.3; \citep{Huffman2001}) and an horizontal line is added to facilitate the comparison with the reference observation (i.e., GPCP v1.3; black).The ensemble members and number are the same as in Figure \ref{fig:portrait_MoV_ampl}.}
    \label{SIfig:MJO_ensembles_summer}
\end{figure}

% %---------------------- FIGURE 10 --------------------------
% \begin{figure}[h]
%     \centering
%     \includegraphics[width=0.8\textwidth]{Paper_figures/Monsoon_Wang2.jpg}
%     \caption{Monsoon metrics obtained from observation datasets (GPCP v1.3 and CMORPH v1.0; \cite{Joyce2004,Xie2017CMORPH} and Historical simulation conducted via NeuralGCM-evap. For each model, we analyzed results for six monsoon regions: all-India rainfall (AIR),  northern Australia (AUS), Sahel, Gulf of Guinea (GoG), North American monsoon (NAMo), and South American monsoon (SAMo).
%     % The regions are defined in \citet{Sperber2014} Metrics for onset (On), duration (Du), and decay (De) derived as differences to the default observation (GPCP v1.3) in pentad indices (observation minus model) are shown at lower right of each panel. 
%     Vertical dashed lines indicate for each region the onset and decay for the obs (black) and the model (red).}
%     \label{SIfig:monsoon_Wang2}
% \end{figure}

%---------------------- FIGURE 10 --------------------------
\begin{figure}[h]
    \centering
    \includegraphics[width=0.7\textwidth]{Paper_figures/Monsoon_NeuralGCM-evap_Sperberg.png}
    \caption{Comparing the precipitation pentads between model and observations in NeuralGCM-evap. The monsoon metrics obtained from observation datasets (GPCP v1.3 and CMORPH v1.0; \cite{Joyce2004,Xie2017CMORPH} and Historical simulation conducted via (a) ACE2 and (b) NeuralGCM-precip. For each model, we analyzed results for six monsoon regions: all-India rainfall (AIR),  northern Australia (AUS), Sahel, Gulf of Guinea (GoG), North American monsoon (NAMo), and South American monsoon (SAMo) for the period 1980-2005.
    % The regions are defined in \citet{Sperber2014} Metrics for onset (On), duration (Du), and decay (De) derived as differences to the default observation (GPCP v1.3) in pentad indices (observation minus model) are shown at lower right of each panel. 
    Vertical dashed lines indicate for each region the onset and decay for the obs (black) and the model (red).}
    \label{SIfig:monsoon_Sper_evap}
\end{figure}

%---------------------- FIGURE 10 --------------------------
\begin{figure}[h]
    \centering
    \includegraphics[width=0.9\textwidth]{Paper_figures/semi-annual.png}
    \caption{Normalized semi-annual precipitation variability with PMP metric in the top right corner of each panel.}
    \label{SIfig:precip_semiannual}
\end{figure}

%---------------------- FIGURE 10 --------------------------
\begin{figure}[h]
    \centering
    \includegraphics[width=0.9\textwidth]{Paper_figures/interannual.png}
    \caption{Normalized interannual precipitation variability with PMP metric in the top right corner of each panel.}
    \label{SIfig:precip_inter}
\end{figure}

% %---------------------- FIGURE 10 --------------------------
% \begin{figure}[h]
%     \centering
%     \includegraphics[width=0.9\textwidth]{Paper_figures/seasonal-annual.png}
%     \caption{Normalized seasonal precipitation variability with PMP metric in the top right corner of each panel.}
%     \label{SIfig:precip_semi}
%     \label{SIfig:seas}
% \end{figure}

% %---------------------- FIGURE 10 --------------------------
% \begin{figure}[h]
%     \centering
%     \includegraphics[width=0.9\textwidth]{Paper_figures/sub-seasonal.png}
%     \caption{Normalized sub-seasonal precipitation variability with PMP metric in the top right corner of each panel.}
%     \label{SIfig:precip_semi}
%     \label{SIfig:subs}
% \end{figure}

% %---------------------- FIGURE 10 --------------------------
% \begin{figure}[h]
%     \centering
%     \includegraphics[width=0.9\textwidth]{Paper_figures/synoptic.png}
%     \caption{Normalized synoptic precipitation variability with PMP metric in the top right corner of each panel.}
%     \label{SIfig:precip_semi}
%     \label{SIfig:syn}
% \end{figure}
